# Supplementary material for: A novel CFA+EFA model to detect aberrant respondents
Source: arXiv:2311.15988 source file (2024-08-07)
Supplement: Supplementary file 1 [file suppl.pdf]

# Supplementary materials for "A novel CFA+EFA model to detect aberrant respondents"

Niccolò Cao[1], Livio Finos[2], Luigi Lombardi[3], Antonio Calcagnì[2]

[1]University of Bologna, [2]University of Padova, [3]University of Trento

## Integration to Simulation study 1

As interestingly suggested by an anonymous reviewer, we investigated how much the magnitude of the inter-item correlations affects the classification performances of the CFA+EFA model.

### *Theoretical considerations*

Theoretically, the strength of the overall inter-item correlations depends mainly on the size of the CFA and EFA errors (respectively, $\text{diag}(\boldsymbol{\Theta}_{\boldsymbol{\delta}})$ and $\text{diag}(\boldsymbol{\Psi}_{\boldsymbol{\epsilon}})$). If the errors of the two FA components are small, the CFA/EFA submodels generally present stronger inter-item correlations, while large errors imply lower correlations. However, from a generative viewpoint, the CFA/EFA models produce different patterns of inter-item correlations. Specifically, the CFA submodel generates stronger correlations among items loading on the same latent variable and weaker correlations among items loading on different latent variables. In contrast, the EFA submodel does not restrict the magnitude of the inter-item correlations. This dissimilarity between CFA and EFA is the keystone of the CFA+EFA model as a classification method (for more details, see Introduction). In this context, varying the overall strength of correlations (i.e., the CFA and EFA errors) should not alter the CFA and EFA patterns of intercorrelations underlying the observed correlation matrix. Therefore, we hypothesized that the magnitude of the overall inter-item correlations may have no impact on the CFA+EFA model's performances.

### *Data analysis and discussion*

To study the relationship between the performances of the CFA+EFA model and the magnitude of inter-item correlations, we employed the data and the results obtained in Simulation study 1. For the sake of simplicity, we considered the conditions with one covariate (i.e., $C = 1$). Then, the design of the study was reduced to 12 conditions by varying only: $\pi = \{0.05, 0.60, 0.90\}$, $q = \{1, 3\}$, and $K = \{2, 4\}$. For each condition, we reconstructed the simulated magnitudes of correlations $r = \{\texttt{stronger}, \texttt{weaker}\}$. By comparing the mean of the observed inter-item correlations for each generated dataset with the mean of the correlations over all the replications, the replications with average correlations under the overall mean were assigned to the

| **Beta regression model** | $\hat{\boldsymbol{\theta}}(\boldsymbol{\sigma}_{\hat{\boldsymbol{\theta}}})$ | $(1-\alpha\%)$CI |
|---|---|---|
| Residual quantiles: Q1:−0.707, Med:0.045, Q3:0.577 | | |
| Location coefficients (logit link): | | |
| $\beta_0$ (Intercept) | 1.408 (0.008) | [1.393; 1.423] |
| $\beta_1$: $\pi$ (`0.05` vs. `0.60`) | 1.300 (0.009) | [1.282; 1.318] |
| $\beta_2$: $\pi$ (`0.05` vs. `0.90`) | 0.876 (0.008) | [0.861; 0.892] |
| $\beta_3$: $K$ (`2` vs. `4`) | −0.011 (0.010) | [−0.030; 0.008] |
| $\beta_4$: $q$ (`1` vs. `3`) | 0.132 (0.010) | [0.113; 0.151] |
| $\beta_5$: $K$ (`2` vs. `4`) : $q$ (`1` vs. `3`) | −0.217 (0.014) | [−0.244; −0.191] |
| Precision coefficients (log link): | | |
| $\gamma_0$ (Intercept) | 4.222 (0.018) | [4.186; 4.258] |
| $\gamma_1$: $r$ (`stronger` vs. `weaker`) | −0.005 (0.025) | [−0.055; 0.044] |
| pseudo-$R^2 = 0.651$ | | |
| $\ell(\boldsymbol{\beta}, \boldsymbol{\gamma}) = 22990.312$ | | |
| AIC $= -45964.62$ | | |

Table 1: Integration to Simulation study 1: Estimates, standard errors, and CIs of the Beta regression model predicting the values of BACC index by the selected factors of the Simulation study 1.

`weaker` condition and vice versa for the `stronger` condition. By doing so, the final design of the study comprised 24 conditions.

Figure 1 reports the boxplots of the classification results for each condition of the design, where red boxplots corresponds to the `weaker` condition and the green ones to the `stronger` condition. Overall, the magnitude of the inter-item correlations seem to have no impact on the classification performances.

To quantitatively assess which factors actually affect the classification results, we predicted the BACC values, which is a comprehensive measure, by the design factors through a Beta regression model, using the `R` package `betareg` (Cribari-Neto & Zeileis, 2010). The Beta model was selected according to a backward stepwise procedure based on the AIC index (Garofalo, 2022), starting from the full model which consists of $\{r, \pi, K, q\}$ as location predictors and $r$ as precision predictor. Table 1 shows the selected Beta regression model, which does not include $r$ as a location predictor but only as a precision predictor with a non-significant coefficient. In conclusion, the magnitude of the inter-item correlations seems to have no impact on the classification performances of the CFA+EFA model.

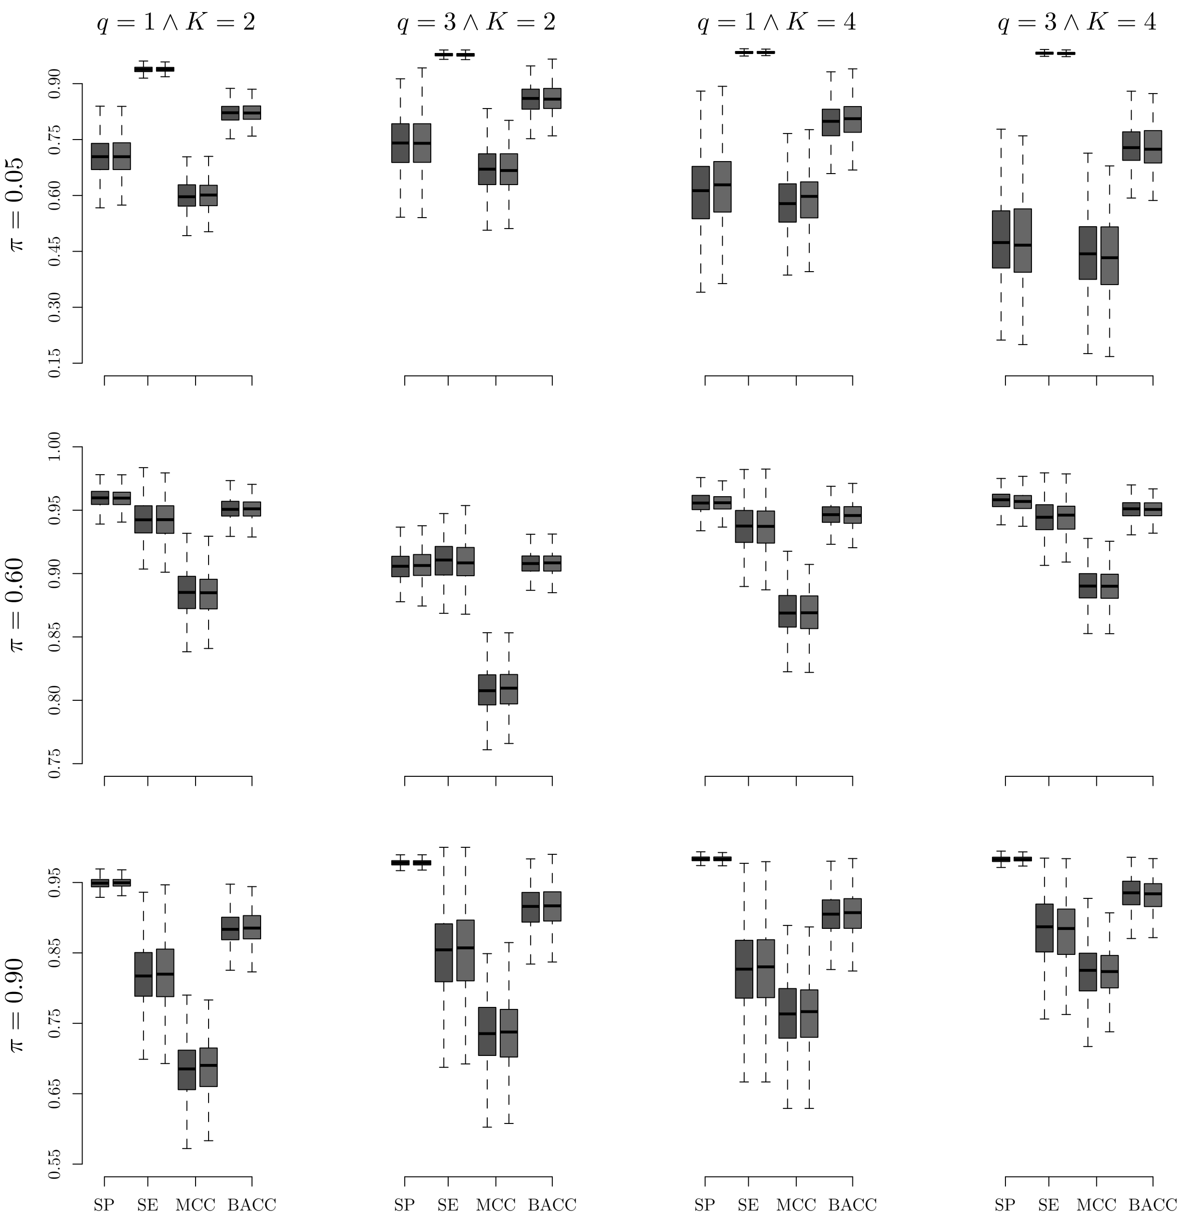


Figure 1: Integration to Simulation study 1: Boxplots of the classification results for the selected conditions of the design. Red boxplots corresponds to the `weaker` condition and the green ones to the `stronger` condition. On the x-axis the classifications indices are reported: specificity (SP), sensitivity (SE), Matthews Correlation Coefficient (MCC), and balanced classification accuracy (BACC).

## Simulation study 3

Considering a general aberrant response style, the aim of this simulation study was twofold. First, we evaluated the accuracy of a set of model selection indices for correctly identifying the true model. To achieve this, we estimated both a correctly specified and a misspecified

CFA+EFA model, where the misspecification was realized by estimating an incorrect number of factors within the EFA component. The whole simulation procedure has been performed on a (remote) HPC machine and the analyses have been completed by using `Julia` software (Bezanson et al., 2017).

**Design** The design of the simulation study involved 3 factors: (i) $\pi \in \{0.40, 0.60, 0.80, 0.90\}$, (ii) $q \in \{1, 3\}$, (iii) $K = \{2, 4\}$. In this study, the true number of EFA latent factors denoted by $K^*$ was set to 4, whereas $K$ represents the number of EFA factors estimated in the CFA+EFA model. The factors were systematically varied in the complete factorial design with a total of $5 \times 2 \times 2 = 20$ scenarios. The invariant inputs for the model were the sample size fixed at 1000 and the number of observed variables $p = 30$. For each combination, $B = 1000$ samples were generated which correspond to $1000 \times 20 = 20000$ new data and the corresponding number of parameters.

**Procedure** Let $q_h$, $\pi_w$, and $k_o$ be different levels of factors $q$, $\pi$, and $K$. Then, the data matrices were generated by:

(a) For $i = 1, \dots, n$, $j = 1, \dots, p$, and $q = 1, \dots, q_l$ the true parameters of the CFA model (Bollen, 1989) were obtained by:

$$\lambda_{1j\times q_l} \sim \mathrm{U}(0.05, 0.99), \quad \boldsymbol{\Phi}_{q_l \times q_l} \sim \mathrm{LKJ}(1, q_l), \quad \boldsymbol{\Lambda}_{1p\times q_l} = \boldsymbol{\Lambda}_{1p\times q_l} \cdot \boldsymbol{\Lambda}^{\text{str}}_{p\times q_l}, \quad \boldsymbol{\mu} = \mathbf{0}_{q_l},$$

$$\boldsymbol{\Theta}_{\boldsymbol{\delta}p\times p} = \mathbf{1}_{p\times 1} - \mathrm{diag}(\boldsymbol{\Lambda}_{p\times q_l} \boldsymbol{\Phi}_{q_l\times q_l} \boldsymbol{\Lambda}^T_{p\times q_l}), \quad \boldsymbol{\nu}_{K^*\times 1} = \mathrm{U}(0.5, 5), \quad \lambda_{2j\times K^*} \sim \mathrm{U}(0.05, 0.99),$$

$$\boldsymbol{\Psi}_{\boldsymbol{\epsilon}p\times p} = 0.85 \cdot \mathbf{I}_{p\times p}, \quad \beta_1 = \log\left(\frac{\pi_w}{(1-\pi_w)}\right), \quad \boldsymbol{\beta}_2 \sim \mathrm{U}(-1.5, 1.5), \quad x_{i,2} \sim \mathcal{B}ern(0.5)$$

where $\mathrm{U}(0.05, 0.99)$ represents the uniform distribution, $\mathrm{LKJ}(1, q)$ indicates the Lewandowski-Kurowicka-Joe distribution with shape parameter equals to 1 and dimension of the extracted factor correlation matrix of $q_l \times q_l$, $\boldsymbol{\Lambda}^{\text{str}}_{p\times q_l}$ is a matrix of zeros and ones which determines the constrained structure of the $\boldsymbol{\Lambda}_{1p\times q_l}$ matrix by linking not overlapping vectors of indicators to distinct latent factors, and the intercept of the logistic regression is represented by $x_{i,1} = 1$.

(b) For $m = 1, \dots, M$ with $M = 50000$, the CFA respondents' latent traits, measurement errors, and continuous vectors of responses were computed as $\boldsymbol{\eta}_{q_l\times m} \sim N_{q_l}(\mathbf{0}_q, \boldsymbol{\Phi}_{q_l\times q_l})$, $\boldsymbol{\delta}_{p\times m} \sim N_p(\mathbf{0}_p, \boldsymbol{\Theta}_{\boldsymbol{\delta}p\times p})$, and $\boldsymbol{y}_{p\times m} = \boldsymbol{\Lambda}_{1p\times q_l}\boldsymbol{\eta}_{q_l\times m} + \boldsymbol{\delta}_{p\times m}$.

(c) For $r = 1, \dots, R$ with $R = 50000$, the EFA respondents' latent traits, measurement errors, and continuous vectors of responses were computed as $\boldsymbol{\xi}_{K^*\times r} \sim N_{K^*}(\mathbf{0}_{K^*}, \boldsymbol{I}_{K^*\times K^*})$, $\boldsymbol{\epsilon}_{p\times r} \sim N_j(\mathbf{0}_p, \boldsymbol{\Psi}_{\boldsymbol{\epsilon}p\times p})$, and $\boldsymbol{y}_{p\times r} = \boldsymbol{\Lambda}_{2p\times K^*}\boldsymbol{\xi}_{K^*\times r} + \boldsymbol{\epsilon}_{p\times r}$.

(d) For $i = 1, \dots, n$ and $d = 2$, the latent indicator variable of the mixture was sampled by: $\pi_{n\times 1} = \frac{\exp(\boldsymbol{X}_{n\times d}\boldsymbol{\beta}_{d\times 1})}{(\exp(\boldsymbol{X}_{n\times d}\boldsymbol{\beta}_{d\times 1}) + \mathbf{1}_{n\times 1})}$ and $\boldsymbol{z}_{n\times 1} \sim \mathcal{B}ern(\pi_{n\times 1})$

(e) The data matrix is obtained by $\boldsymbol{Y}_{p\times n} = [\{\boldsymbol{y}_{p\times m} \mid \boldsymbol{z}_{i\times 1} = \mathbf{1}_{i\times 1}\}, \{\boldsymbol{y}_{p\times r} \mid \boldsymbol{z}_{i\times 1} = \mathbf{0}_{i\times 1}\}]^T$.

(f) The generated data matrix of $\boldsymbol{Y}_{p\times n}$ was analysed using the CFA+EFA model using $k_o$ as the number of EFA factors.

**Model selection indices.** The information criteria (IC) and classification criteria (CC) are popular methods for model selection in the framework of FMMs (Cintron et al., 2023; Henson et al., 2007; Jedidi et al., 1997; McLachlan & Peel, 2000). We tested the accuracy of the following statistics (Henson et al., 2007; McLachlan & Peel, 2000): Akaike Information Criterion (AIC), consistent Akaike Information Criterion (CAIC), Bayesian Information Criterion (BIC), sample-adjusted BIC (ssBIC), Classification Likelihood Information Criterion (CLC), Integrated Classification Likelihood-BIC (ICL-BIC), and entropy (H). The formulae used:

$$\text{AIC} = 2d - 2\ell(\mathbf{\Omega}), \quad \text{CAIC} = d\left(\log(n) + 1\right) - 2\ell(\mathbf{\Omega}), \quad \text{BIC} = d\log(n) - 2\ell(\mathbf{\Omega}),$$
$$\text{ssBIC} = \log\left(\frac{n+2}{24}\right) d - 2\ell(\mathbf{\Omega}), \quad \text{CLC} = 2E - 2\ell(\mathbf{\Omega}),$$
$$\text{ICL-BIC} = 2E + \log(n)d - 2\ell(\mathbf{\Omega}), \quad \text{H} = 1 - \frac{E}{n\log(G)}$$

where, $\ell(\mathbf{\Omega})$ is the log-likelihood function of the CFA+EFA model parameters $\mathbf{\Omega}$, $d$ is the number of estimated parameter for the model, $n$ is the sample size, $G$ is the number of components (i.e., $G = 2$ in our case), and the statistic $E$ is computed as:

$$E = -\sum_{g=1}^{G}\sum_{i=1}^{n} f(z_{ig} = 1 \mid \boldsymbol{y}_i; \mathbf{\Omega}) \log\left(f(z_{ig} = 1 \mid \boldsymbol{y}_i; \mathbf{\Omega})\right)$$

where, $z_{ig} \in \{0, 1\}$ indicates the classification variable for the observation $i$ to the component $g$, $\boldsymbol{y}_i$ is the observed vector of the manifest variables, $f(z_i = g \mid \boldsymbol{y}_i; \mathbf{\Omega})$ represents the posterior probability of the observation's $i$ membership to the component $g$.

Table 2: Monte Carlo study: percentages of the correct model selection procedure based on Akaike Information Criterion (AIC), consistent Akaike Information Criterion (CAIC), Bayesian Information Criterion (BIC), sample-adjusted BIC (ssBIC), Classification Likelihood Information Criterion (CLC), Integrated Classification Likelihood-BIC (ICL-BIC), and entropy (H).

| $\pi$ | $q$ | AIC | CAIC | BIC | ssBIC | CLC | ICL-BIC | H |
|---|---|---|---|---|---|---|---|---|
| 0.40 | 1 | 100.0 | 100.0 | 100.0 | 100.0 | 100.0 | 100.0 | 99.6 |
| | 3 | 6.9 | 6.3 | 6.3 | 6.8 | 7.0 | 6.4 | 18.7 |
| 0.60 | 1 | 100.0 | 100.0 | 100.0 | 100.0 | 100.0 | 100.0 | 100.0 |
| | 3 | 82.7 | 61.4 | 65.8 | 76.5 | 87.4 | 65.8 | 58.5 |
| 0.80 | 1 | 99.4 | 94.2 | 95.6 | 98.5 | 99.9 | 96.7 | 99.9 |
| | 3 | 64.9 | 64.9 | 64.9 | 64.9 | 65.0 | 64.9 | 100.0 |
| 0.90 | 1 | 0.0 | 0.0 | 0.0 | 0.0 | 0.0 | 0.0 | 93.7 |
| | 3 | 91.8 | 89.6 | 90.3 | 91.4 | 92.3 | 90.7 | 99.8 |

**Results and discussion** Table 2 shows the percentages of Monte Carlo replications for which the indices correctly selected the true model over the misspecified one. In particular, the percentages of correct selection of the model with $K = 4$ against the misspecified one with $K = 2$ are reported. For $\boldsymbol{\pi}$, higher accuracy is observed for proportions such as $\{0.60, 0.80, 0.90\}$. This corroborates the use of these indices for model selection in the applied contexts for which

the model is intended for. Considering $\boldsymbol{q}$, the percentages are generally higher under conditions with $q = 1$. However, it interesting to note that all the indices completely failed to recover the true model in the case of $\pi = 0.90$ and $q = 1$ but entropy, which reported a satisfying performance. Overall, the indices demonstrated similar performances except for the entropy index, which consistently exhibited the best recovery rates.

# Table S1

| Model | $\ell$ | AIC | CAIC | BIC | ssBIC | CLC | ICL-BIC | H |
|---|---|---|---|---|---|---|---|---|
| $K = 1$ | −28877.941 | 58053.881 | 58882.685 | 58733.685 | 58260.575 | 57916.328 | 58894.132 | 0.837 |
| $K = 2$ | −30519.953 | 61411.906 | 62446.52 | 62260.52 | 61669.927 | 61226.147 | 62446.761 | 0.81 |
| $K = 3$ | −30505.757 | 61457.514 | 62697.939 | 62474.939 | 61766.862 | 61216.547 | 62679.972 | 0.791 |
| $K = 4$ | −30238.754 | 60997.508 | 62443.743 | 62183.743 | 61358.183 | 60546.167 | 62252.403 | 0.93 |
| $K = 5$ | −31107.771 | 62809.541 | 64461.587 | 64164.587 | 63221.543 | 62235.4 | 64184.446 | 0.98 |
| $K = 6$ | −30056.708 | 60781.416 | 62639.272 | 62305.272 | 61244.744 | 60170.618 | 62362.474 | 0.942 |
| $K = 7$ | −28562.659 | 57867.318 | 59930.985 | 59559.985 | 58381.973 | 57234.696 | 59669.362 | 0.889 |
| $K = 8$ | −30553.681 | 61923.363 | 64192.84 | 63784.84 | 62489.345 | 61208.602 | 63886.08 | 0.897 |
| $K = 9$ | −30605.38 | 62100.761 | 64576.048 | 64131.048 | 62718.07 | 61303.344 | 64223.632 | 0.906 |
| $K = 10$ | −31489.177 | 63942.355 | 66623.453 | 66141.453 | 64610.99 | 62979.413 | 66142.511 | 0.999 |
| $K = 11$ | −30651.245 | 62340.491 | 65227.399 | 64708.399 | 63060.453 | 61302.529 | 64708.437 | 1.0 |
| $K = 12$ | −28787.229 | 58686.458 | 61779.177 | 61223.177 | 59457.747 | 57709.905 | 61358.624 | 0.862 |
| $K = 13$ | −30312.022 | 61810.044 | 65108.573 | 64515.573 | 62632.66 | 60638.511 | 64530.041 | 0.985 |
| $K = 14$ | −30172.996 | 61605.993 | 65110.332 | 64480.332 | 62479.936 | 60345.995 | 64480.335 | 1.0 |
| $K = 15$ | −30216.694 | 61767.388 | 65477.538 | 64810.538 | 62692.658 | 60463.08 | 64840.23 | 0.97 |
| $K = 16$ | −29781.424 | 60970.848 | 64886.808 | 64182.808 | 61947.444 | 59564.187 | 64184.148 | 0.999 |
| $K = 17$ | −30098.029 | 61678.057 | 65799.828 | 65058.828 | 62705.981 | 60199.602 | 65062.373 | 0.996 |
| $K = 18$ | −30344.454 | 62244.908 | 66572.489 | 65794.489 | 63324.158 | 60688.918 | 65794.499 | 1.0 |
| $K = 19$ | −29375.975 | 60381.95 | 64915.342 | 64100.342 | 61512.527 | 58752.05 | 64100.442 | 1.0 |
| $K = 20$ | −30180.78 | 62065.56 | 66804.762 | 65952.762 | 63247.464 | 60378.902 | 65970.105 | 0.982 |
| $K = 1 \wedge$ gender | −30149.642 | 60601.283 | 61441.212 | 61290.212 | 60810.752 | 60454.703 | 61445.632 | 0.842 |
| $K = 2 \wedge$ gender | −30098.992 | 60573.983 | 61619.723 | 61431.723 | 60834.779 | 60341.78 | 61575.519 | 0.853 |
| $K = 3 \wedge$ gender | −29849.102 | 60148.205 | 61399.755 | 61174.755 | 60460.327 | 59783.436 | 61259.986 | 0.913 |
| $K = 4 \wedge$ gender | −30694.156 | 61912.312 | 63369.672 | 63107.672 | 62275.761 | 61489.84 | 63209.2 | 0.897 |
| $K = 5 \wedge$ gender | −28580.055 | 57758.11 | 59421.28 | 59122.28 | 58172.886 | 57285.685 | 59247.855 | 0.872 |
| $K = 6 \wedge$ gender | −29793.736 | 60259.472 | 62128.453 | 61792.453 | 60725.575 | 59677.081 | 61882.062 | 0.909 |
| $K = 7 \wedge$ gender | −31434.23 | 63614.461 | 65689.252 | 65316.252 | 64131.891 | 62868.47 | 65316.261 | 1.0 |
| $K = 8 \wedge$ gender | −30394.258 | 61608.516 | 63889.118 | 63479.118 | 62177.272 | 60856.094 | 63546.696 | 0.931 |
| $K = 9 \wedge$ gender | −30638.963 | 62171.927 | 64658.339 | 64211.339 | 62792.01 | 61370.535 | 64303.948 | 0.906 |
| $K = 10 \wedge$ gender | −30869.652 | 62707.305 | 65399.528 | 64915.528 | 63378.715 | 61815.534 | 64991.757 | 0.922 |
| $K = 11 \wedge$ gender | −30559.644 | 62161.287 | 65059.321 | 64538.321 | 62884.024 | 61120.426 | 64539.459 | 0.999 |
| $K = 12 \wedge$ gender | −30946.484 | 63008.969 | 66112.813 | 65554.813 | 63783.033 | 61896.925 | 65558.769 | 0.996 |
| $K = 13 \wedge$ gender | −31973.121 | 65136.242 | 68445.896 | 67850.896 | 65961.632 | 64010.968 | 67915.622 | 0.934 |
| $K = 14 \wedge$ gender | −30390.099 | 62044.198 | 65559.663 | 64927.663 | 62920.916 | 60800.606 | 64948.07 | 0.979 |
| $K = 15 \wedge$ gender | −30171.913 | 61681.826 | 65403.102 | 64734.102 | 62609.871 | 60353.928 | 64744.203 | 0.99 |
| $K = 16 \wedge$ gender | −30109.511 | 61631.022 | 65558.108 | 64852.108 | 62610.394 | 60219.419 | 64852.505 | 1.0 |
| $K = 17 \wedge$ gender | −29623.409 | 60732.819 | 64865.715 | 64122.715 | 61763.517 | 59246.819 | 64122.715 | 1.0 |
| $K = 18 \wedge$ gender | −29937.38 | 61434.76 | 65773.466 | 64993.466 | 62516.785 | 59877.497 | 64996.204 | 0.997 |
| $K = 19 \wedge$ gender | −29966.526 | 61567.053 | 66111.569 | 65294.569 | 62700.404 | 59934.107 | 65295.624 | 0.999 |
| $K = 20 \wedge$ gender | −29977.138 | 61662.276 | 66412.603 | 65558.603 | 62846.954 | 59974.439 | 65578.767 | 0.979 |
| $K = 1 \wedge$ age | −29696.995 | 59693.991 | 60528.357 | 60378.357 | 59902.072 | 59549.561 | 60533.928 | 0.841 |
| $K = 2 \wedge$ age | −30519.388 | 61412.777 | 62452.954 | 62265.954 | 61672.185 | 61223.372 | 62450.549 | 0.812 |
| $K = 3 \wedge$ age | −30503.498 | 61454.996 | 62700.984 | 62476.984 | 61765.731 | 61211.213 | 62681.2 | 0.792 |
| $K = 4 \wedge$ age | −29599.435 | 59720.87 | 61172.667 | 60911.667 | 60082.932 | 59350.692 | 61063.49 | 0.845 |
| $K = 5 \wedge$ age | −30240.527 | 61077.054 | 62734.662 | 62436.662 | 61490.443 | 60544.01 | 62499.619 | 0.936 |
| $K = 6 \wedge$ age | −31669.093 | 64008.186 | 65871.604 | 65536.604 | 64472.901 | 63338.532 | 65536.951 | 1.0 |
| $K = 7 \wedge$ age | −30901.899 | 62547.798 | 64617.028 | 64245.028 | 63063.841 | 61803.8 | 64245.029 | 1.0 |
| $K = 8 \wedge$ age | −29771.022 | 60360.045 | 62635.084 | 62226.084 | 60927.414 | 59543.47 | 62227.509 | 0.999 |
| $K = 9 \wedge$ age | −30488.513 | 61869.027 | 64349.877 | 63903.877 | 62487.723 | 60983.119 | 63909.969 | 0.994 |
| $K = 10 \wedge$ age | −30588.455 | 62142.91 | 64829.57 | 64346.57 | 62812.933 | 61176.91 | 64346.57 | 1.0 |
| $K = 11 \wedge$ age | −30475.449 | 61990.898 | 64883.369 | 64363.369 | 62712.248 | 60951.192 | 64363.663 | 1.0 |
| $K = 12 \wedge$ age | −30186.005 | 61486.01 | 64584.292 | 64027.292 | 62258.687 | 60372.01 | 64027.292 | 1.0 |
| $K = 13 \wedge$ age | −31174.332 | 63536.664 | 66840.756 | 66246.756 | 64360.668 | 62396.513 | 66294.604 | 0.951 |
| $K = 14 \wedge$ age | −30286.381 | 61834.762 | 65344.664 | 64713.664 | 62710.092 | 60575.365 | 64716.268 | 0.997 |
| $K = 15 \wedge$ age | −30189.018 | 61714.037 | 65429.749 | 64761.749 | 62640.694 | 60382.483 | 64766.196 | 0.995 |
| $K = 16 \wedge$ age | −29899.651 | 61209.302 | 65130.826 | 64425.826 | 62187.286 | 59806.17 | 64432.693 | 0.993 |
| $K = 17 \wedge$ age | −30129.788 | 61743.575 | 65870.909 | 65128.909 | 62772.886 | 60271.182 | 65140.516 | 0.988 |
| $K = 18 \wedge$ age | −29579.083 | 60716.166 | 65049.31 | 64270.31 | 61796.803 | 59158.166 | 64270.31 | 1.0 |
| $K = 19 \wedge$ age | −30271.118 | 62174.235 | 66713.19 | 65897.19 | 63306.2 | 60577.048 | 65932.003 | 0.965 |
| $K = 20 \wedge$ age | −29512.164 | 60730.328 | 65475.093 | 64622.093 | 61913.619 | 59025.395 | 64623.16 | 0.999 |
| $K = 1 \wedge$ gender $\wedge$ age | −30149.642 | 60601.283 | 61441.212 | 61290.212 | 60810.752 | 60454.703 | 61445.632 | 0.842 |
| $K = 2 \wedge$ gender $\wedge$ age | −30098.992 | 60573.983 | 61619.723 | 61431.723 | 60834.779 | 60341.78 | 61575.519 | 0.853 |
| $K = 3 \wedge$ gender $\wedge$ age | −29849.102 | 60148.205 | 61399.755 | 61174.755 | 60460.327 | 59783.436 | 61259.986 | 0.913 |
| $K = 4 \wedge$ gender $\wedge$ age | −30694.156 | 61912.312 | 63369.672 | 63107.672 | 62275.761 | 61489.84 | 63209.2 | 0.897 |
| $K = 5 \wedge$ gender $\wedge$ age | −28580.055 | 57758.11 | 59421.28 | 59122.28 | 58172.886 | 57285.685 | 59247.855 | 0.872 |
| $K = 6 \wedge$ gender $\wedge$ age | −29793.736 | 60259.472 | 62128.453 | 61792.453 | 60725.575 | 59677.081 | 61882.062 | 0.909 |
| $K = 7 \wedge$ gender $\wedge$ age | −31434.23 | 63614.461 | 65689.252 | 65316.252 | 64131.891 | 62868.47 | 65316.261 | 1.0 |
| $K = 8 \wedge$ gender $\wedge$ age | −30394.258 | 61608.516 | 63889.118 | 63479.118 | 62177.272 | 60856.094 | 63546.696 | 0.931 |
| $K = 9 \wedge$ gender $\wedge$ age | −30638.963 | 62171.927 | 64658.339 | 64211.339 | 62792.01 | 61370.535 | 64303.948 | 0.906 |
| $K = 10 \wedge$ gender $\wedge$ age | −30869.652 | 62707.305 | 65399.528 | 64915.528 | 63378.715 | 61815.534 | 64991.757 | 0.922 |
| $K = 11 \wedge$ gender $\wedge$ age | −30559.644 | 62161.287 | 65059.321 | 64538.321 | 62884.024 | 61120.426 | 64539.459 | 0.999 |
| $K = 12 \wedge$ gender $\wedge$ age | −30946.484 | 63008.969 | 66112.813 | 65554.813 | 63783.033 | 61896.925 | 65558.769 | 0.996 |
| $K = 13 \wedge$ gender $\wedge$ age | −31973.121 | 65136.242 | 68445.896 | 67850.896 | 65961.632 | 64010.968 | 67915.622 | 0.934 |
| $K = 14 \wedge$ gender $\wedge$ age | −30390.099 | 62044.198 | 65559.663 | 64927.663 | 62920.916 | 60800.606 | 64948.07 | 0.979 |
| $K = 15 \wedge$ gender $\wedge$ age | −30171.913 | 61681.826 | 65403.102 | 64734.102 | 62609.871 | 60353.928 | 64744.203 | 0.99 |
| $K = 16 \wedge$ gender $\wedge$ age | −30109.511 | 61631.022 | 65558.108 | 64852.108 | 62610.394 | 60219.419 | 64852.505 | 1.0 |
| $K = 17 \wedge$ gender $\wedge$ age | −29623.409 | 60732.819 | 64865.715 | 64122.715 | 61763.517 | 59246.819 | 64122.715 | 1.0 |
| $K = 18 \wedge$ gender $\wedge$ age | −29937.38 | 61434.76 | 65773.466 | 64993.466 | 62516.785 | 59877.497 | 64996.204 | 0.997 |
| $K = 19 \wedge$ gender $\wedge$ age | −29966.526 | 61567.053 | 66111.569 | 65294.569 | 62700.404 | 59934.107 | 65295.624 | 0.999 |
| $K = 20 \wedge$ gender $\wedge$ age | −29977.138 | 61662.276 | 66412.603 | 65558.603 | 62846.954 | 59974.439 | 65578.767 | 0.979 |

# A Appendix: EM algorithm

In a mixture modelling context, the direct maximization of the observed data log-likelihood $\ell(\boldsymbol{\Omega};\boldsymbol{y})$ is complicated (see for instance Bishop and Nasrabadi, 2006). However, we can maximize the complete-data log-likelihood $\ell(\boldsymbol{\Omega};\boldsymbol{y},\boldsymbol{u})$ by using the EM algorithm to obtain Maximum Likelihood (ML) estimation.

Our EM algorithm requires to be initialized by plugging-in a set of random starting values for the parameters $\boldsymbol{\Omega}^0$. Let $\boldsymbol{\Omega}' = \boldsymbol{\Omega}^{(t-1)}$ be the $(t-1)$-th estimates of $\boldsymbol{\Omega}$, the EM procedure performs the following first two steps for each iteration $t$:

1. **E-step**: compute $\mathbb{E}_{\boldsymbol{\Omega}'}\left[\ell\left(\boldsymbol{\Omega};\boldsymbol{y};\boldsymbol{u}\right) \mid \boldsymbol{y}_i, \hat{\boldsymbol{\Omega}}'\right]$
2. **M-step**: solve $\hat{\boldsymbol{\Omega}}^t = \arg\max_{\boldsymbol{\Omega}} \mathbb{E}_{\boldsymbol{\Omega}'}\left[\ell\left(\boldsymbol{\Omega};\boldsymbol{y};\boldsymbol{u}\right) \mid \boldsymbol{y}_i, \hat{\boldsymbol{\Omega}}'\right]$
3. Convergence if $\epsilon' > \left|\mathbb{E}_{\boldsymbol{\Omega}'}\left[\ell\left(\boldsymbol{\Omega};\boldsymbol{y};\boldsymbol{u}\right) \mid \boldsymbol{y}_i, \hat{\boldsymbol{\Omega}}'\right] - \mathbb{E}_{\boldsymbol{\Omega}'}\left[\ell\left(\boldsymbol{\Omega};\boldsymbol{y};\boldsymbol{u}\right) \mid \boldsymbol{y}_i, \hat{\boldsymbol{\Omega}}'\right]\right|$

## A.1 E-step

In the E-step, we need to compute the expected value of the joint log-likelihood of the observed and latent data given the observed data, which corresponds to:

$$
\begin{aligned}
\mathbb{Q}\left(\boldsymbol{\Omega} \mid \hat{\boldsymbol{\Omega}}'\right) &= \mathbb{E}_{\boldsymbol{\Omega}'}\left[\ell\left(\boldsymbol{\Omega};\boldsymbol{y};\boldsymbol{x}\right) \mid \boldsymbol{y}_i, \hat{\boldsymbol{\Omega}}'\right] \\
&= \sum_{i=1}^{n} \mathbb{E}_{\boldsymbol{\Omega}'}\left[z_i = 1 \mid \boldsymbol{y}_i\right] \left\{ \log(\hat{\pi}_i') - \frac{(p+q)}{2}\log(2\pi) - \frac{1}{2}\log\left(\mid \hat{\boldsymbol{\Theta}}'_{\boldsymbol{\delta}} \mid\right) - \right. \\
&- \frac{1}{2}\log\left(\mid \hat{\boldsymbol{\Phi}}' \mid\right) - \frac{n}{2} trace\left[\hat{\boldsymbol{\Theta}}'^{-1}_{\boldsymbol{\delta}}\left(\frac{1}{n}\boldsymbol{y}_i\boldsymbol{y}_i^T - 2\frac{1}{n}\boldsymbol{y}_i\hat{\boldsymbol{\Lambda}}_1'^T\mathbb{E}_{\boldsymbol{\Omega}'}[\boldsymbol{\eta}_i \mid \boldsymbol{y}_i]^T + \right.\right. \\
&+ \left.\left.\frac{1}{n}\hat{\boldsymbol{\Lambda}}_1'\mathbb{E}_{\boldsymbol{\Omega}'}[\boldsymbol{\eta}_i\boldsymbol{\eta}_i^T \mid \boldsymbol{y}_i]\boldsymbol{\Lambda}_1'^T\right)\right] - \frac{n}{2} trace\left[\hat{\boldsymbol{\Phi}}'^{-1}\left(\frac{1}{n}\mathbb{E}_{\boldsymbol{\Omega}'}[\boldsymbol{\eta}_i\boldsymbol{\eta}_i^T \mid \boldsymbol{y}_i] - \right.\right. \\
&- \left.\left.\left.\frac{2}{n}\mathbb{E}_{\boldsymbol{\Omega}'}[\boldsymbol{\eta}_i \mid \boldsymbol{y}_i]\hat{\boldsymbol{\mu}}'^T + \frac{1}{n}\hat{\boldsymbol{\mu}}'\hat{\boldsymbol{\mu}}'^T\right)\right]\right\} + \sum_{i=1}^{n}\mathbb{E}_{\boldsymbol{\Omega}'}[z_i = 0 \mid \boldsymbol{y}_i]\left\{\log(1-\hat{\pi}_i') - \right. \\
&- \frac{(p+K)}{2}\log(2\pi) - \frac{1}{2}\log\left(\mid \hat{\boldsymbol{\Psi}}'_{\boldsymbol{\epsilon}} \mid\right) - \frac{n}{2} trace\left[\hat{\boldsymbol{\Psi}}'^{-1}_{\boldsymbol{\epsilon}}\left(\frac{1}{n}\boldsymbol{y}_i\boldsymbol{y}_i^T - \right.\right. \\
&- \left.\left. 2\hat{\boldsymbol{\Lambda}}_2'\mathbb{E}_{\boldsymbol{\Omega}'}\left[\boldsymbol{\xi}_i \mid \boldsymbol{y}_i\right]\frac{1}{n}\boldsymbol{y}_i^T + \frac{1}{n}\boldsymbol{\Lambda}_2'\mathbb{E}_{\boldsymbol{\Omega}'}[\boldsymbol{\xi}_i\boldsymbol{\xi}_i^T \mid \boldsymbol{y}_i]\hat{\boldsymbol{\Lambda}}_2'^T\right)\right] - \\
&- \left.\frac{n}{2} trace\left(\frac{1}{n}\mathbb{E}_{\boldsymbol{\Omega}'}[\boldsymbol{\xi}_i\boldsymbol{\xi}_i^T \mid \boldsymbol{y}_i] - \frac{2}{n}\mathbb{E}_{\boldsymbol{\Omega}'}\left[\boldsymbol{\xi}_i \mid \boldsymbol{y}_i\right]\hat{\boldsymbol{\nu}}'^T + \frac{1}{n}\hat{\boldsymbol{\nu}}'\hat{\boldsymbol{\nu}}'^T\right)\right\}
\end{aligned}
\tag{1}
$$

The conditional expected values of the sufficient statistics for the array of parameters $\boldsymbol{\Omega}$ given the data and the current parameter values are computed as follows:

$$
\mathbb{E}_{\boldsymbol{\Omega}'}[S_{\boldsymbol{z}=1} \mid \boldsymbol{y}] = \sum_{i=1}^{n}\mathbb{E}_{\boldsymbol{\Omega}'}[z_i = 1 \mid \boldsymbol{y}_i] \tag{2}
$$

$$\mathbb{E}_{\boldsymbol{\Omega}'}[S_{\boldsymbol{z}=0} \mid \boldsymbol{y}] = \sum_{i=1}^{n} \mathbb{E}_{\boldsymbol{\Omega}'}[z_i = 0 \mid \boldsymbol{y}_i] \tag{3}$$

$$\mathbb{E}_{\boldsymbol{\Omega}'}[S_{\boldsymbol{y}}^{(\boldsymbol{z}=1)} \mid \boldsymbol{y}] = \frac{1}{n} \sum_{i=1}^{n} \mathbb{E}_{\boldsymbol{\Omega}'}[z_i = 1 \mid \boldsymbol{y}_i] \boldsymbol{y}_i \tag{4}$$

$$\mathbb{E}_{\boldsymbol{\Omega}'}[S_{\boldsymbol{y}}^{(\boldsymbol{z}=0)} \mid \boldsymbol{y}] = \frac{1}{n} \sum_{i=1}^{n} \mathbb{E}_{\boldsymbol{\Omega}'}[z_i = 0 \mid \boldsymbol{y}_i] \boldsymbol{y}_i \tag{5}$$

$$\mathbb{E}_{\boldsymbol{\Omega}'}[S_{\boldsymbol{y}\boldsymbol{y}^T}^{(\boldsymbol{z}=1)} \mid \boldsymbol{y}] = \frac{1}{n} \sum_{i=1}^{n} \mathbb{E}_{\boldsymbol{\Omega}'}[z_i = 1 \mid \boldsymbol{y}_i] \boldsymbol{y}_i \boldsymbol{y}_i^T \tag{6}$$

$$\mathbb{E}_{\boldsymbol{\Omega}'}[S_{\boldsymbol{y}\boldsymbol{y}^T}^{(\boldsymbol{z}=0)} \mid \boldsymbol{y}] = \frac{1}{n} \sum_{i=1}^{n} \mathbb{E}_{\boldsymbol{\Omega}'}[z_i = 0 \mid \boldsymbol{y}_i] \boldsymbol{y}_i \boldsymbol{y}_i^T \tag{7}$$

$$\mathbb{E}_{\boldsymbol{\Omega}'}[S_{\boldsymbol{\eta}} \mid \boldsymbol{y}] = \frac{1}{n} \sum_{i=1}^{n} \mathbb{E}_{\boldsymbol{\Omega}'}[z_i = 1 \mid \boldsymbol{y}_i] \mathbb{E}_{\boldsymbol{\Omega}'}[\boldsymbol{\eta}_i \mid \boldsymbol{y}_i] \tag{8}$$

$$\mathbb{E}_{\boldsymbol{\Omega}'}[S_{\boldsymbol{\xi}} \mid \boldsymbol{y}] = \frac{1}{n} \sum_{i=1}^{n} \mathbb{E}_{\boldsymbol{\Omega}'}[z_i = 0 \mid \boldsymbol{y}_i] \mathbb{E}_{\boldsymbol{\Omega}'}[\boldsymbol{\xi}_i \mid \boldsymbol{y}_i] \tag{9}$$

$$\mathbb{E}_{\boldsymbol{\Omega}'}[S_{\boldsymbol{y}\boldsymbol{\eta}^T} \mid \boldsymbol{y}] = \frac{1}{n} \sum_{i=1}^{n} \mathbb{E}_{\boldsymbol{\Omega}'}[z_i = 1 \mid \boldsymbol{y}_i] \boldsymbol{y}_i \mathbb{E}_{\boldsymbol{\Omega}'}[\boldsymbol{\eta}_i^T \mid \boldsymbol{y}_i] \tag{10}$$

$$\mathbb{E}_{\boldsymbol{\Omega}'}[S_{\boldsymbol{y}\boldsymbol{\xi}^T} \mid \boldsymbol{y}] = \frac{1}{n} \sum_{i=1}^{n} \mathbb{E}_{\boldsymbol{\Omega}'}[z_i = 0 \mid \boldsymbol{y}_i] \boldsymbol{y}_i \mathbb{E}_{\boldsymbol{\Omega}'}[\boldsymbol{\xi}_i^T \mid \boldsymbol{y}_i] \tag{11}$$

$$\mathbb{E}_{\boldsymbol{\Omega}'}[S_{\boldsymbol{\eta}\boldsymbol{\eta}^T} \mid \boldsymbol{y}] = \frac{1}{n} \sum_{i=1}^{n} \mathbb{E}_{\boldsymbol{\Omega}'}[z_i = 1 \mid \boldsymbol{y}_i] \mathbb{E}_{\boldsymbol{\Omega}'}[\boldsymbol{\eta}_i \mid \boldsymbol{y}_i] \mathbb{E}_{\boldsymbol{\Omega}'}[\boldsymbol{\eta}_i^T \mid \boldsymbol{y}_i] \tag{12}$$

$$\mathbb{E}_{\boldsymbol{\Omega}'}[S_{\boldsymbol{\xi}\boldsymbol{\xi}^T} \mid \boldsymbol{y}] = \frac{1}{n} \sum_{i=1}^{n} \mathbb{E}_{\boldsymbol{\Omega}'}[z_i = 0 \mid \boldsymbol{y}_i] \mathbb{E}_{\boldsymbol{\Omega}'}[\boldsymbol{\xi}_i \mid \boldsymbol{y}_i] \mathbb{E}_{\boldsymbol{\Omega}'}[\boldsymbol{\xi}_i^T \mid \boldsymbol{y}_i] \tag{13}$$

where, the conditional expected values of the CFA and EFA components given the data are derived by applying the properties of the conditional multivariate Normal distribution (Azzalini, 1996):

$$\mathbb{E}_{\boldsymbol{\Omega}'}[\boldsymbol{\eta}_i \mid \boldsymbol{y}_i] = \hat{\boldsymbol{\mu}}' + \hat{\boldsymbol{\Phi}}' \hat{\boldsymbol{\Lambda}}_1'^T \left( \hat{\boldsymbol{\Lambda}}_1' \hat{\boldsymbol{\Phi}}' \hat{\boldsymbol{\Lambda}}_1'^T + \hat{\boldsymbol{\Theta}}_{\delta}' \right)^{-1} \left( \boldsymbol{y}_i - \hat{\boldsymbol{\Lambda}}_1' \hat{\boldsymbol{\mu}}' \right) \tag{14}$$

$$\mathbb{E}_{\boldsymbol{\Omega}'}[\boldsymbol{\eta}_i \boldsymbol{\eta}_i^T \mid \boldsymbol{y}_i] = \hat{\boldsymbol{\Phi}}' - \hat{\boldsymbol{\Phi}}' \hat{\boldsymbol{\Lambda}}_1'^T \left( \hat{\boldsymbol{\Lambda}}_1' \hat{\boldsymbol{\Phi}}' \hat{\boldsymbol{\Lambda}}_1'^T + \hat{\boldsymbol{\Theta}}_{\delta}' \right)^{-1} \hat{\boldsymbol{\Lambda}}_1' \hat{\boldsymbol{\Phi}}' + \mathbb{E}_{\boldsymbol{\Omega}'}[\boldsymbol{\eta}_i \mid \boldsymbol{y}_i] \mathbb{E}_{\boldsymbol{\Omega}'}[\boldsymbol{\eta}_i \mid \boldsymbol{y}_i]^T \tag{15}$$

$$\mathbb{E}_{\boldsymbol{\Omega}'}[\boldsymbol{\xi}_i \mid \boldsymbol{y}_i] = \hat{\boldsymbol{\nu}}' + \hat{\boldsymbol{\Lambda}}_2'^T \left( \hat{\boldsymbol{\Lambda}}_2' \hat{\boldsymbol{\Lambda}}_2'^T + \hat{\boldsymbol{\Psi}}_{\delta}' \right)^{-1} \left( \boldsymbol{y}_i - \hat{\boldsymbol{\Lambda}}_2' \hat{\boldsymbol{\nu}}' \right) \tag{16}$$

$$\mathbb{E}_{\boldsymbol{\Omega}'}[\boldsymbol{\xi}_i \boldsymbol{\xi}_i^T \mid \boldsymbol{y}_i] = \boldsymbol{I}_K - \hat{\boldsymbol{\Lambda}}_2'^T \left( \hat{\boldsymbol{\Lambda}}_2' \hat{\boldsymbol{\Lambda}}_2'^T + \hat{\boldsymbol{\Psi}}_{\delta}' \right)^{-1} \hat{\boldsymbol{\Lambda}}_2' + \mathbb{E}_{\boldsymbol{\Omega}'}[\boldsymbol{\xi}_i \mid \boldsymbol{y}_i] \mathbb{E}_{\boldsymbol{\Omega}'}[\boldsymbol{\xi}_i \mid \boldsymbol{y}_i]^T \tag{17}$$

and the conditional expected values of the classification latent variable given the observed data

are computed as:

$$\mathbb{E}_{\boldsymbol{\Omega}'}[z_i = 1 \mid \boldsymbol{y}_i] = \frac{\hat{\pi}_i' \mathcal{N}_p(\boldsymbol{y}_i; \hat{\boldsymbol{\Lambda}}_1' \hat{\boldsymbol{\mu}}', \hat{\boldsymbol{\Lambda}}_1' \hat{\boldsymbol{\Phi}}' \hat{\boldsymbol{\Lambda}}_1'^T + \hat{\boldsymbol{\Theta}}_{\boldsymbol{\delta}}')}{\hat{\pi}_i' \mathcal{N}_p(\boldsymbol{y}_i; \hat{\boldsymbol{\Lambda}}_1' \hat{\boldsymbol{\mu}}', \hat{\boldsymbol{\Lambda}}_1' \hat{\boldsymbol{\Phi}}' \hat{\boldsymbol{\Lambda}}_1'^T + \hat{\boldsymbol{\Theta}}_{\boldsymbol{\delta}}') + (1 - \hat{\pi}_i') \mathcal{N}_p(\boldsymbol{y}_i; \hat{\boldsymbol{\Lambda}}_2' \hat{\boldsymbol{\nu}}', \hat{\boldsymbol{\Lambda}}_2' \hat{\boldsymbol{\Lambda}}_2'^T + \hat{\boldsymbol{\Psi}}_{\boldsymbol{\delta}})} \tag{18}$$

$$\mathbb{E}_{\boldsymbol{\Omega}'}[z_i = 0 \mid \boldsymbol{y}_i] = 1 - \mathbb{E}_{\boldsymbol{\Omega}'}[z_i = 1 \mid \boldsymbol{y}_i] \tag{19}$$

## A.2 M-step

Once computed the sufficient statistics in the E-step, the M-step consists in maximizing $\mathbb{Q}(\hat{\boldsymbol{\Omega}} \mid \hat{\boldsymbol{\Omega}}')$ with respect to the elements of $\boldsymbol{\Omega}$ and it can be completed by plugging-in Equations (2)-(13) into the complete log-likelihood Equation (1). In the M-step, by setting the score functions equal to zero, we obtain the maximum likelihood estimates for the $t$-th iteration of the EM:

$$\hat{\boldsymbol{\Lambda}}_1' = \frac{\mathbb{E}_{\boldsymbol{\Omega}'}[S_{\boldsymbol{y}\boldsymbol{\eta}^T} \mid \boldsymbol{y}]}{\mathbb{E}_{\boldsymbol{\Omega}'}[S_{\boldsymbol{\eta}\boldsymbol{\eta}^T} \mid \boldsymbol{y}]} \tag{20}$$

$$\hat{\boldsymbol{\Theta}}_{\boldsymbol{\delta}}' = \frac{\mathbb{E}_{\boldsymbol{\Omega}'}[S_{\boldsymbol{y}\boldsymbol{y}^T}^{(\boldsymbol{z}=1)} \mid \boldsymbol{y}] - \hat{\boldsymbol{\Lambda}}_1' \mathbb{E}_{\boldsymbol{\Omega}'}[S_{\boldsymbol{y}\boldsymbol{\eta}^T} \mid \boldsymbol{y}]}{\mathbb{E}_{\boldsymbol{\Omega}'}[S_{\boldsymbol{z}=1} \mid \boldsymbol{y}]/n} \tag{21}$$

$$\hat{\boldsymbol{\mu}}' = \frac{\mathbb{E}_{\boldsymbol{\Omega}'}[S_{\boldsymbol{\eta}} \mid \boldsymbol{y}]}{\mathbb{E}_{\boldsymbol{\Omega}'}[S_{\boldsymbol{z}=1} \mid \boldsymbol{y}]} \tag{22}$$

$$\hat{\boldsymbol{\Phi}}' = \frac{\mathbb{E}_{\boldsymbol{\Omega}'}[S_{\boldsymbol{\eta}\boldsymbol{\eta}^T} \mid \boldsymbol{y}] - \hat{\boldsymbol{\mu}}'^T \mathbb{E}_{\boldsymbol{\Omega}'}[S_{\boldsymbol{\eta}} \mid \boldsymbol{y}]}{\mathbb{E}_{\boldsymbol{\Omega}'}[S_{\boldsymbol{z}=1} \mid \boldsymbol{y}]/n} \tag{23}$$

$$\hat{\boldsymbol{\Lambda}}_2' = \frac{\mathbb{E}_{\boldsymbol{\Omega}'}[S_{\boldsymbol{y}\boldsymbol{\xi}^T} \mid \boldsymbol{y}]}{\mathbb{E}_{\boldsymbol{\Omega}'}[S_{\boldsymbol{\xi}\boldsymbol{\xi}^T} \mid \boldsymbol{y}]} \tag{24}$$

$$\hat{\boldsymbol{\Psi}}_{\boldsymbol{\epsilon}}' = \frac{\mathbb{E}_{\boldsymbol{\Omega}'}[S_{\boldsymbol{y}\boldsymbol{y}^T}^{(\boldsymbol{z}=0)} \mid \boldsymbol{y}] - \hat{\boldsymbol{\Lambda}}_2' \mathbb{E}_{\boldsymbol{\Omega}'}[S_{\boldsymbol{y}\boldsymbol{\xi}^T} \mid \boldsymbol{y}]}{\mathbb{E}_{\boldsymbol{\Omega}'}[S_{\boldsymbol{z}=0} \mid \boldsymbol{y}]/n} \tag{25}$$

$$\hat{\boldsymbol{\nu}}' = \frac{\mathbb{E}_{\boldsymbol{\Omega}'}[S_{\boldsymbol{\xi}} \mid \boldsymbol{y}]}{\mathbb{E}_{\boldsymbol{\Omega}'}[S_{\boldsymbol{z}=0} \mid \boldsymbol{y}]} \tag{26}$$

$$\hat{\pi}' = \frac{\mathbb{E}_{\boldsymbol{\Omega}'}[S_{\boldsymbol{z}=1} \mid \boldsymbol{y}]}{n} \tag{27}$$

However, if covariates $\boldsymbol{X}$ (matrix $n \times C+1$) are included in the mixture parameter $\pi$ through the logit link, the ML estimates can not be derived through a closed-form expression for the covariate parameters $\boldsymbol{\beta}$, as the score function of $\boldsymbol{\beta}$, $\mathbf{g}(\hat{\boldsymbol{\beta}})$, is a nonlinear function:

$$\frac{\partial \mathbb{Q}(\boldsymbol{\Omega} \mid \boldsymbol{\Omega}')}{\partial \boldsymbol{\beta}} = -\boldsymbol{X}^T \left\{ \left[ \mathbb{E}_{\boldsymbol{\Omega}'}[\boldsymbol{z} = 1 \mid \boldsymbol{y}_i] - \mathbb{E}_{\boldsymbol{\Omega}'}[\boldsymbol{z} = 0 \mid \boldsymbol{y}_i] \exp(\boldsymbol{X}\hat{\boldsymbol{\beta}}) \right] \left[ \mathbf{1} + \exp(\boldsymbol{X}\hat{\boldsymbol{\beta}}) \right]^{-1} \right\} \tag{28}$$

Therefore, a Newton-Raphson method has been applied by employing the Hessian matrix:

$$\mathbf{H}(\hat{\boldsymbol{\beta}}) = -\boldsymbol{X}^T \left\{ \exp(\boldsymbol{X}\hat{\boldsymbol{\beta}}) \left[ \mathbf{1} + \exp(\boldsymbol{X}\hat{\boldsymbol{\beta}}) \right]^{-2} \right\} \boldsymbol{X} \tag{29}$$

In particular, an iteration $v$ of this method is given by:

$$\hat{\boldsymbol{\beta}}^{(v,t)} = \hat{\boldsymbol{\beta}}^{(v,t)} - \mathbf{H}^{-1} \left( \hat{\boldsymbol{\beta}}^{(v-1,t)} \right) \mathbf{g} \left( \hat{\boldsymbol{\beta}}^{(v-1,t)} \right) \tag{30}$$

## References


Azzalini, A. (1996). *Statistical inference based on the likelihood* (Vol. 68). CRC Press.

Bezanson, J., Edelman, A., Karpinski, S., & Shah, V. B. (2017). Julia: A fresh approach to numerical computing. *SIAM Review*, *59*(1), 65–98.

Bishop, C. M., & Nasrabadi, N. M. (2006). *Pattern recognition and machine learning* (Vol. 4). Springer.

Bollen, K. A. (1989). *Structural equations with latent variables*. John Wiley & Sons.

Cintron, D. W., Loken, E., & McCoach, D. B. (2023). A cautionary note about having the right mixture model but classifying the wrong people. *Multivariate Behavioral Research*, *58*(4), 675–686.

Cribari-Neto, F., & Zeileis, A. (2010). Beta regression in r. *Journal of Statistical Software*, *34*(2), 1–24. https://doi.org/10.18637/jss.v034.i02

Garofalo, S. (2022). *Stepbeta: Stepwise procedure for beta, beta-binomial and negative binomial regression models* [R package version 2.1.0]. https://CRAN.R-project.org/package=StepBeta

Held, L., & Sabanés Bové, D. (2014). *Applied statistical inference*. Springer.

Henson, J. M., Reise, S. P., & Kim, K. H. (2007). Detecting mixtures from structural model differences using latent variable mixture modeling: A comparison of relative model fit statistics. *Structural Equation Modeling: A Multidisciplinary Journal*, *14*(2), 202–226.

Jedidi, K., Jagpal, H. S., & DeSarbo, W. S. (1997). Stemm: A general finite mixture structural equation model. *Journal of Classification*, *14*(1), 23–50.

McLachlan, G. J., & Peel, D. (2000). *Finite mxiture models*. John Wiley & Sons.
